# Supplementary material for: Multi-Task Multi-Scale Contrastive Knowledge Distillation for Efficient Medical Image Segmentation
Source: arXiv:2406.03173 source file (2024-06-05)
Supplement: Supplementary file 1 [file A_AppA.tex]

%~~~~~~~~~~~~~~~~~~~~~~~~~~~~~~~~~~~~~~~~~~~~~~~~~~~~~~~~~~~~~~~~~~~~~~~~~~~~~~~~~~~~~~~~~%
%                                    APPENDIX TEMPLATE                                    %
%~~~~~~~~~~~~~~~~~~~~~~~~~~~~~~~~~~~~~~~~~~~~~~~~~~~~~~~~~~~~~~~~~~~~~~~~~~~~~~~~~~~~~~~~~%

% Use these after the \appendix command at the end of report.tex
% Appendices work similar to a chapter and are used to provide supplementary information that typically do not contribute to the final page count of a report.

\chapter{Long Appendix Title Here} % Main appendix title

\label{AppendixA} % for referencing this appendix elsewhere, use \ref{AppendixA}

% This is for the header on each page if in use - input a shortened title due to constrictions.
% \lhead{Appendix A. \emph{Short App. Title Here}}

Write your Appendix content here. Sections and subsections can be used as well.
\section{First Appendix Section}
\subsection{First Appendix Subsection}
\subsubsection{First Appendix Subsubsection}
Appendices will show up in the ToC numbered as letters. This is of course totally customizable, please refer to the CTAN documentation (\url{https://ctan.org/pkg/appendix?lang=en}) for further clarity on the same.
